# Supplementary material for: Towards pandemic preparedness: ability to estimate high-resolution social contact patterns from longitudinal surveys
Source: arXiv:2411.03774 source file (2024-11-06)
Supplement: Supplementary file 1 [file supp_methods_old.tex]

\subsection*{Identifying individual-level factors associated with the number of daily social contacts and reporting fatigue.}
%
We here describe our approach to identifying factors associated with the number of daily social contacts and reporting fatigue associated with repeat survey participation. Let $Y^0_i$ for $i = 1,2,\ldots, n_0$ and $Y^1_i$ for $i = 1,2,\ldots, n_1$ denote the number of contacts by a first-time participant and a repeating participant, respectively. We implemented a two-stage variable selection process where the variables relevant to the number of daily social contacts are selected in the first stage using data from first-time participants, and those variables further associated with reporting fatigue are identified in the second stage. The COVIMOD survey included two waves with a good balance of first-time participants and repeating participants, waves 4 and waves 21. We identified variables associated with the number of daily social contacts and reporting fatigue first on wave 4, and then tested if the same variables were also identified in wave 21 to assess the robustness in variable selection procedures. The final selected variables were the union of the selected variables from both waves. A complete list of candidate variables and selection results can be found in Table~\ref{tab:varselect-variables}. 

In the first stage, we analysed data from first-time participants and considered the model
\begin{subequations}\label{eq:stage-1-varselect}
\begin{align}
    Y^0_i &\sim \text{Poisson}(\lambda_i) \quad \text{for } i = 1,2,\ldots,n_0 \\
    \log(\lambda_i) &= \beta_0 + \bm{u}^\top_i \alpha + \bm{v}^\top_i \beta
\end{align}
\end{subequations}
where $\bm{u}_i$ is a vector consisting of covariates that are well-established for their association with heterogeneity in count intensities (gender, age, household size)~\cite{wong_social_2023, dan_estimating_2023, backer_contact_2024,  gimma_changes_2022, tomori_individual_2021, loedy_longitudinal_2023}, and $\bm{v}_i$ is a vector of further putative covariates that could be associated with heterogeneity in count intensities, which we tested through regularised horseshoe (RHS) variable selection~\cite{piironen_sparsity_2017}. We assigned generic un-informative priors to $\beta_0$ and $\alpha = (\alpha_1, \alpha_2, \ldots, \alpha_J)^\top$, 
\begin{align*}
    \beta_0 &\sim \text{Normal}(0, 100) \\
    \alpha_j &\sim \text{Normal}(0, \sigma^2_\alpha) \quad j = 1,2,\ldots,J \\
    \sigma_\alpha &\sim \text{half-Cauchy}^+(0, 1),
\end{align*}
and RHS priors to $\beta = (\beta_1, \beta_2, \ldots, \beta_K)^\top$,
\begin{subequations}\label{eq:horseshoe-prior}
\begin{align}
\beta_k | \zeta_k, \varepsilon, c &\sim \text{Normal}(0, \varepsilon^2\tilde{\zeta}_k^2), \quad \tilde{\zeta}_k^2 = \frac{c^2\zeta_k^2}{c^2 + \varepsilon^2\zeta^2_k}\label{eq:horseshoe-prior-a} \\
\zeta_k &\sim \text{student-}t^+_{\nu_1}(0,1), \quad k = 1,\ldots,K \\
c^2 &\sim \text{Gamma}(\nu_2, \nu_2 s^2/2) \\
\varepsilon &\sim \text{student-}t^+_{\nu_3}(0, \varepsilon_0),
\end{align}
\end{subequations}
where the scaling parameter $\varepsilon_0$ for $\varepsilon$ was expressed as 
\begin{equation*}
    \varepsilon_0 = \frac{p_0}{P-p_0} \frac{1}{n},
\end{equation*}
with $P$ the number of covariates in the model and $p_0 \in \{0, \dotsc, K\}$ specified to reflect prior knowledge on the effective number of non-zero coefficients~\cite{piironen_sparsity_2017}. For succinctness, we denote this prior as
\begin{equation*}
    \beta_k \sim \text{RHS}_{\nu_1,\nu_2,\nu_3}(s^2, p_0).
\end{equation*}
We set the hyperparameters of the RHS prior to $\nu_1 = 3, \nu_2 = 2, \nu_3 = 4, s^2 = 2$ to facilitate sampling in {\it Stan}~\cite{piironen_sparsity_2017}, and $p_0 = K/2$ to obtain a weakly informative prior on the number of selected variables. Following inference, variables were retained if the absolute medium effect size of their corresponding coefficient was less than or greater than $\log(1.05) \approx 0.049$, which corresponds to a 5\% change from the population average contact rate $\exp(\beta_0)$. We performed a sensitivity analysis where $p0$ was set to 1 (strong shrinkage) or $K - 1$ (weak shrinkage). Both settings did not change the features that were selected.

In the second stage, we retained the selected coefficients and investigated the presence of reporting fatigue on the data from repeating participants through the model
\begin{subequations}\label{eq:stage-2-varselect}
\begin{align}
    Y^1_i &\sim \text{Poisson}(\lambda_i) \quad \text{for } i = 1,2,\ldots,n_1 \\
    \log(\lambda_i) &= \hat\beta_0 + \bm{u}^\top_i \hat{\alpha} + \bm{v}^\top_i \hat{\beta}+ \bm{w}^\top_i \gamma, 
\end{align}
\end{subequations}
where $\hat\beta_0$, $\hat{\alpha}$, and $\hat{\beta}$ denote the posterior median point estimates from model~\eqref{eq:stage-1-varselect} fitted to data from first-time participants (without using the RHS prior), and $\bm{w}_i$ is a vector consisting of covariates putatively associated with reporting fatigue. As fatigue should only have negative effects on contact intensity, we constrained $\bm{\gamma}$ to only take negative values. This was done by replacing  Eq.~\eqref{eq:horseshoe-prior-a} with a half-normal prior such that $\gamma_l | \zeta_l, \varepsilon, c \sim \text{half-Normal}^{-}(0, (1-2/\pi)^{-1} \varepsilon^2 \tilde{\zeta}^2_l)$ for $l = 1,2,\ldots,L$. For simplicity, we denote the constrained RHS prior as
\begin{equation}
    \gamma_l \sim \text{half-RHS}^{-}_{\nu_1,\nu_2,\nu_3}(s^2, p_0).
\end{equation}
The adjustment factor $(1-2/\pi)^{-1}$ in the scale component of the half normal was added to ensure that the prior variance of the constrained RHS prior is equivalent to that of the non-constrained version. As in the first-stage analysis, we set the hyperparameters of the RHS prior to $\nu_1 = 3, \nu_2 = 2, \nu_3 = 4, s^2 = 2$~\cite{piironen_sparsity_2017}, and $p_0 = L/2$. All inference in this work was performed using the \textit{Stan}\cite{stan_development_team_stan_2022} probabilistic programming language through the \textit{cmdstanr}\cite{jonah_gabry_cmdstanr_2023} package version 2.34.1 as front-end. 

\subsection*{Investigating the functional form of reporting fatigue effects over the number of repeat participations}
Here, we describe our approach to identifying the functional form of reporting fatigue with the number of times individuals participate in the study. Let $Y_{i,r}$ denote the number of contacts reported by individual $i$ in their $r$-th participation, with $i=1,\dotsc,N$ and $r=0,1,\dotsc,R$. Additionally, we introduce the index map $t_{i,r}$ that identifies the wave that individual $i$ had at their $r$-th participation. For instance, if the third repeat ($r = 3$) of the first participant ($i=1$) was reported during the $4$-th wave, then $t_{i,r} =  4$. $Y_{i,0}$ corresponds to the number of contacts reported the first-time that individual $i$ participated in the study. Further, let $\bm{x}_{i,r} = (x_{i,1}, \ldots, x_{i,J})^\top$ denote a $J$ dimensional vector containing the covariates selected in the previous variable selection analysis along with age, gender, and household size.

We assessed increasingly less complex Bayesian Negative Binomial count models in their ability to describe mean trends in $Y_{i,r}$, and all these models had the following common components, 
\begin{subequations}\label{eq:longitudinal-model}
\begin{align}
 Y_{i,r} &\sim \text{NegBinomial}(\lambda_{i,r}, \varphi) \\
\log(\lambda_{i,r}) &= \beta_0 + \bm{x}_{i,r}^\top\beta + \tau(t_{i,r}) + \rho(r) \\
\tau(t) &\sim \text{GP}(0, k),   
\end{align}
\end{subequations}
where $\varphi$ denotes a real-valued overdispersion parameter such that the mean and variance of the Negative Binomial observation model are $\E{Y_{i,r}} = \lambda_{i,r}$ and $\Var{Y_{i,r}} = \lambda_{i,r} + \lambda_{i,r}^2/\varphi$. The latent random variable $\alpha$ is the baseline term, and $\beta = (\beta_1, \ldots, \beta_J)^\top$ is a vector of coefficients for the individuals' characteristics, and calendar-time effects are modelled as deviations from the baseline $\alpha$ through a zero-mean Gaussian process characterised by the Mat\'ern 3/2 covariance kernel
\begin{equation}
k(t, t')  = \sigma_{\tau} \left(1 + \frac{\sqrt{3}|t - t'|}{\ell_\tau} \right) \exp\left( -\frac{\sqrt{3}|t - t'|}{\ell_\tau} \right).  
\end{equation}
Throughout, we used the following generic priors to the parameters in the components common across all models:
\begin{subequations}
\begin{align}
1/\varphi &\sim \text{Exponential}(1), \\
\beta_0 &\sim \text{Normal}(0, 10), \\
\beta_j &\overset{i.i.d}{\sim} \text{Normal}(0, \sigma^2_{\beta}) \quad j = 1,\ldots,J \\
\sigma_{\beta} &\sim \text{Cauchy}^+(0,1) \\
\sigma_{\tau}, \ell_{\tau} &\overset{i.i.d.}{\sim} \text{inv-Gamma}(5, 1).
\end{align}
\end{subequations}
We considered three different approaches for capturing the functional form on how  reporting fatigue accumulates with the number of repeat participation. The first model comprised $R$ independent reporting fatigue effects 
\begin{equation}
    \rho_r \overset{i.i.d.}{\sim} \text{Normal}(0, 1) \quad r \in \{1,2,\ldots,R\},
\end{equation}
with $\rho_{r=0}$ set to $0$ for identifiability. This first model imposes no specific functional form of reporting fatigue with $r$. The second model was a non-parametric Gaussian process prior with squared exponential kernel depending on rescaled repeat times $\tilde{r} = (r - \text{mean})/\text{sd-dev}$
\begin{subequations}
\begin{align}
    \rho^{\text{GP}}(\tilde{r}) & \sim \text{GP}(0, k_{\text{SE}})\\
    k_{\text{SE}}(\tilde{r},\tilde{r}') & = \sigma_\rho \exp\left( -\frac{(\tilde{r}-\tilde{r}')^2}{2 \ell_\rho^2} \right) \\
    \sigma_{\rho}, \ell_{\rho} &\overset{i.i.d.}{\sim} \text{inv-Gamma}(5, 1)
\end{align}
\end{subequations}
for $r=1,\dotsc,R$, and $\rho^{\text{GP}}=0$ for $r=0$ to ensure identifiability. This model imposes smooth trends on reporting fatigue effects with the number of repeat participations, and consequently renders reporting fatigue effects more predictable.
\begin{figure}
    \centering
    \includegraphics{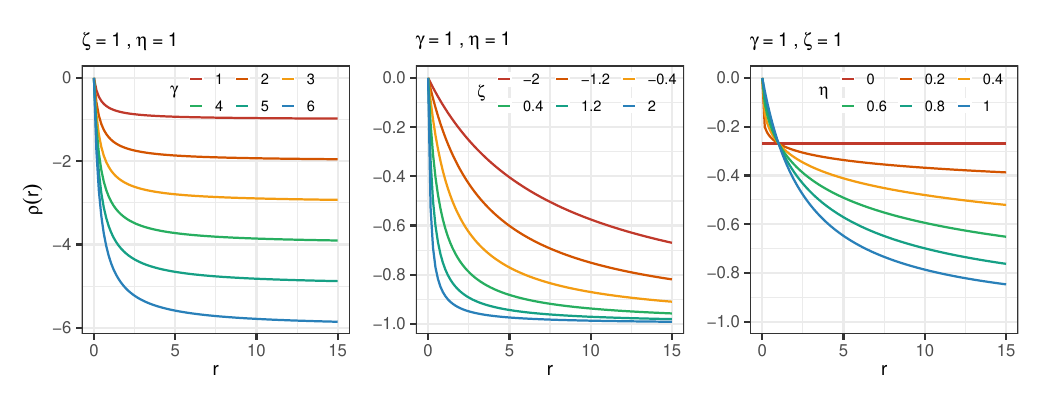}
    \caption{Functional form of the Hill function under different parameter values.}
    \label{fig:hill-function}
\end{figure}
For the third model, we take inspiration from dose-response modeling in biochemistry~\cite{prinz_hill_2009} and model reporting fatigue with a three-parameter Hill function:
\begin{equation}\label{eq:hill-function}
    \rho^{\text{Hill}}(r) = -\gamma \frac{e^\zeta r^\eta}{1 + e^\zeta r^\eta} \quad \text{where} \quad \gamma, \eta \in \mathbb{R}^+, \zeta \in \mathbb{R}
\end{equation}
where $\gamma$ is a scale parameter which control the effect size at large values of $r$, while $\zeta$ and $\eta$ in tandem controls how quickly the function approaches its minimum value. Figure~\ref{fig:hill-function} shows the functional form of the Hill function under different parameter values. This model is computationally more efficient than GP models, and renders due to its parametric form reporting fatigue effects strongly predictable. Given their constraints, we assign the following priors to each parameter:
\begin{align*}
    \gamma &\sim \text{half-Normal}^+(0,1) \\
    \zeta &\sim \text{Normal}(0,1) \\
    \eta &\sim \text{Exponential}(1).
\end{align*}

\subsection*{Generalised additive model for fine-age contact intensity with reporting fatigue adjustment}
 %Now, we merge the insights from the two previous models to estimate marginal social contact intensities from data potentially corrupted by reporting fatigue. We selected data from COVIMOD wave 21, which includes a mix of first-time and multiple-time participants, and was collected after the second wave of COVID-19 lockdowns in Germany, minimizing the impact of contact reduction measures on our analysis.

%Our objectives are twofold: the first is to validate a method for correcting the effects of reporting fatigue in existing datasets, and second is to determine the threshold of participant repeats beyond which fatigue significantly skews the data, despite statistical corrections. We begin by splitting the data based on the participants' number of repeats. We fit a model on a subset of the data with only first-time participants, and treat the estimates we obtain as the reference or \textit{pseudo-truth}. We then add back the splits containing participants with repeats in an incremental fashion, assessing at each step the mean square error (MSE) and the proportion of estimates within the 95\% confidence interval (CI) relative to the psuedo-truth. This approach helps us evaluate how well our adjustment works and identify the maximum number of repeat participation we can include before data reliability declines. The following text details the construction of our proposed model.

Let $a_i$ denote the age of participant, $\bm{u}_i = (u_{i1}, \ldots, u_{iP})^\top \in \{0,1\}^P$ denote the vector of gender and household size variables, and $\bm{w}_i = (w_{i1}, \ldots, w_{iQ})^\top \in \{0,1\}^Q$ denote the vector of covariates associated with reporting fatigue identified in the variable selection analysis. We consider the following negative binomial generalised additive count model,
\begin{subequations} \label{eq:gam}
\begin{align}
    Y_{i,r} &\sim \text{NegBinomial}\left( \lambda_{i,r}, \varphi \right), \\
    \log(\lambda_{i,r}) &= \beta_0 + \bm{u}_i^\top \beta + f_\theta(a_i) + \bm{w}^\top_i \rho(r)
\end{align}
\end{subequations}
where $\beta_0$ is a global baseline parameter and $\rho(r) \in \mathbb{R}^Q$ is a vector consisting of elements
\begin{align*}
    [\rho(r)]_q = -\gamma_q \exp(\zeta_q)r^{\eta_q}/(1+\exp(\zeta_q)r^{\eta_q})
\end{align*}
which models the fatigue effect at each repeat for the selected variables.
$\alpha$ and the covariate parameter vector $\beta = (\beta_1, \beta_2, \ldots, \beta_p)^\top$ are assigned generic Gaussian priors, and the reciprocal of the overdispersion parameter $\varphi$ is given an exponential prior:
\begin{align*}
    \beta_0 &\sim \text{Normal}(0, 10), \\
    \beta_p &\overset{i.i.d.}{\sim} \text{Normal}(0, 1), \quad p = 1,\ldots,P \\
    1/\varphi &\sim \text{Exp}(1).
\end{align*}
Let $\hat\gamma, \hat\zeta$, and $\hat\eta$ denote the posterior median estimates from Eq.~\ref{eq:longitudinal-model}. Leveraging the Bayesian framework to reflect prior knowledge, we assign the following informative priors to the parameters of the hill function,
\begin{align*}
    \gamma_q &\overset{i.i.d.}{\sim} \text{half-Normal}^+(\hat\gamma, 0.5), \\
    \zeta_q &\overset{i.i.d.}{\sim} \text{Normal}(\hat\zeta, 0.1), \\
    \eta_q &\overset{i.i.d.}{\sim} \text{half-Normal}^+(\hat\eta, 0.1).
\end{align*}
$f_\theta(a_i): \mathbb{R} \mapsto \mathbb{R}$ is a non-linear function that describes the effect of participant age on the rate of contact. For computational efficiency, $f_\theta$ is modeled using the zero-mean Hilbert space approximate Gaussian process~\cite{solin_hilbert_2020, riutort-mayol_practical_2022} (HSGP) which is parametrised by $\theta = (\sigma, \ell)$ and characterised by the squared exponential covariance kernel:
\begin{equation*}
    k(x, x') = \sigma \exp\left( -\frac{(x - x')^2}{2\ell^2} \right).
\end{equation*}

\subsection*{Fatigue adjusted estimates for all waves of COVIMOD}
To obtain fatigue adjusted estimates for all 33 waves of the COVIMOD surveys, we applied the GAM described in the previous section (Eq.~\ref{eq:gam}) in the following manner. Let $t = 1,2,\ldots,33$ be an index for the waves. For the first wave ($t = 1$), priors were unchanged from those defined in the previous section. From the second wave onwards, priors for the parameters of the individual covariates and hill functions were set as,
\begin{align*}
    \beta_{t,p} \sim \text{Normal}(\hat\beta_{t-1,p}, 0.3) \quad \text{for } p = 1,2,\ldots,P
\end{align*}
and
\begin{align*}
    \gamma_{t,q} &\sim \text{half-Normal}^+(\hat\gamma_{t-1,q}, 0.3) \\
    \zeta_{t,q} &\sim \text{Normal}(\hat\zeta_{t-1,q}, 0.1) \\
    \eta_{t,q} &\sim \text{half-Normal}^+(\hat\eta_{t-1,q}, 0.1) \quad \text{for } q = 1,2,\ldots,Q.
\end{align*}
Here, $\hat\beta_{t-1,p}, \hat\gamma_{t-1,q}, \hat\zeta_{t-1,q}$, and $\hat\eta_{t-1,q}$ denote the posterior mean of the parameters from the previous wave. This sequential fitting process allows the model to partially leverage information from previous waves to resolve an un-identifiability issue between $\beta_{t,p}$ and the parameters of the Hill function when there are no first-time participants in the data. For the model based fatigue unadjusted estimates, this identifiability issue did not exist and hence estimates were obtained by fitting the model independently to data from each wave. 
